# Supplementary material for: Towards Motion Forecasting with Real-World Perception Inputs: Are End-to-End Approaches Competitive?
Source: arXiv:2306.09281 source file (2024-03-05)
Supplement: Supplementary file 1 [file supp.tex]

\newpage
\appendix
\section{--- Supplementary Materials (\textcolor{red}{TO REMOVE})---} 
\textcolor{red}{TO REMOVE}
\section{More Experiments with Detection and Tracking}
\subsection{Performance with real-world inputs breakdown}
\label{subsec:breakdown}
Information extracted from perception modules can exhibit various imperfections. 
This may include misdetections (false negatives: FN), where certain agents are not correctly identified or missed entirely. This can typically occur in scenarios with adverse weather conditions or for distant agents and objects \cite{michaelis2019dragon,dong2023benchmarking}. 
Conversely, there can be hallucinations (false positives: FP), where the perception system mistakenly detects scene elements or agents that do not actually exist.
Identity switches (IDS) are another common issue, resulting in tracking errors where the system may mistakenly associate the past trajectory of one agent with another.

In \autoref{tab:real_world_results_per_class}, we break down the analysis of tracking and prediction metrics according to the three object classes: car, bus and truck, in order to highlight different or similar behaviors. The results are also grouped by model category: camera-based models, LiDAR-based models and ground-truth models. It appears that LiDAR-based models lead to the best tracking metrics for the car and the bus class, not for the truck class. Even if there are slight variations, CenterPoint \cite{yin2021center} and VoxelNext \cite{chen2023voxelnext} seem to be robust models considering the overall performance.
\begin{table*}[ht]
\centering

\tabcolsep=0.11cm
    \caption{\yihongh{Detailed forecasting results using AgentFormer \cite{yuan2021agentformer} and LaPred \cite{kim2021lapred} with real-world perception inputs.}}
    \vspace{-2mm}
    \resizebox{\linewidth}{!}{
    \begin{tabular}{c l| c c c c c | c c c c | c c c c}
    \toprule
     & & \multicolumn{5}{c|}{Tracking metrics} & \multicolumn{8}{c}{Forecasting metrics} \\
    \midrule 
      & & & & & & & \multicolumn{4}{c}{AgentFormer \cite{yuan2021agentformer}} & \multicolumn{4}{c}{LaPred \cite{kim2021lapred}} \\
    \midrule
     & Method & MOTA $\uparrow$ & MOTP $\downarrow$ & FP $\downarrow$ & FN $\downarrow$ & IDS $\downarrow$  & AP$_f$ $\uparrow$  & minADE $\downarrow$ & minFDE$\downarrow$ &  MR $\downarrow$ & AP$_f$ $\uparrow$  & minADE $\downarrow$ & minFDE$\downarrow$ &  MR $\downarrow$\\ [0.5ex]
     \midrule
     \parbox[t]{3mm}{\multirow{10}{*}{\rotatebox[origin=c]{90}{Car}}} &   MUTR3D R50 \cite{zhang2022mutr3d} (CVPRW2022)        &  0.221 & 0.562 & 1329 & 5057 & 18 & 0.086  & 3.836  & 6.897  & 0.449 & 0.257	&	2.183&	3.506&	0.174 \\

     &  MUTR3D R101 \cite{zhang2022mutr3d} (CVPRW2022)                                                                          & 0.258 & 0.513 & 1002  & 5092 & 8  & 0.102 &  3.351 & 6.084  &  0.434&0.304	&		1.834	&2.992&	\underline{0.146}\\
     
     &  ViP3D Det\&Track \cite{gu2023vip3d} (CVPR2023)                                                                           & 0.189 & 0.583 & 1365 & 5300 & 3 & 0.117  & 2.358  & \underline{4.330} & \underline{0.342} & 0.236		&	1.989&	3.117	&0.150\\
     
     &  UniAD Det\&Track \cite{uniad} (CVPR2023)                                                                                 & 0.227 & 0.438 & \underline{950} & 5391 & 18 & 0.140  & 2.483 & 4.529  & 0.372 & 0.278		&	2.093	&3.399&	0.164\\

       \cmidrule(){2-15}

    &  MegVii \cite{zhu2019class}+AB3DMOT \cite{Weng2020_AB3DMOT} (IROS2020)    & 0.281 & 0.289 & 1239 & 4601 & 73 & 0.144  & 2.289 & 4.337  & 0.368 & 0.282	&		2.099&	3.525	&0.165\\
    
     &  CenterPoint \cite{yin2021center} (CVPR2021)                              & \underline{0.398} & \underline{0.221} & {1377} & \underline{3570} & 4 & \underline{0.163}  &  \underline{2.107} &  4.363 & 0.412 & \underline{0.406}		&	\underline{1.571}	&\underline{2.797}	&0.148\\
     
     &  VoxelNext \cite{chen2023voxelnext} (CVPR2023)                            & {0.376} & 0.241 & 1367 & {3765} &\underline{ 1} & 0.158  & 2.108  &  4.363 & 0.416 & 0.388	&		1.664&	2.928&	0.166\\

     \cmidrule(){2-15}
      & GT position and identity         & 0.987 & 0.000 & 103 & 0 & 0 &   0.375 &  1.874 & 3.935  & 0.349 & 0.756		&	1.211&2.305&	0.115 \\
     
     &  GT position + Tracking model \cite{yin2021center}      & 0.971 & 0.001 & 135 & 0 & 103 & 0.368 & 1.915  & 3.970  & 0.351 &0.737	&		1.324&	2.464&	0.122 \\
     \midrule
     \parbox[t]{3mm}{\multirow{10}{*}{\rotatebox[origin=c]{90}{Bus}}} &   MUTR3D R50 \cite{zhang2022mutr3d} (CVPRW2022)        & 0.160 & 0.961 & 165 & 404 & 7 & 0.038  &  4.060 & 7.141 & 0.505 & 0.173	&		2.490&	3.578	&0.183\\

     &  MUTR3D R101 \cite{zhang2022mutr3d} (CVPRW2022)                                                                          & 0.268 & 0.818 & 110 & 391 & 1 & 0.060  &  3.228 & 5.983  & 0.482 & 0.255		&	2.020	&2.867&	0.144\\
     
     &  ViP3D Det\&Track \cite{gu2023vip3d} (CVPR2023)                                                                           & 0.121 & 1.018 & 197 & 406 & \underline{0} & 0.043  & 2.853  & 5.083  & 0.466 &0.173		&	2.132	&3.007&	0.144 \\
     
     &  UniAD Det\&Track \cite{uniad} (CVPR2023)                                                                                 & 0.108 & 0.689 & 130 & 480 & 2 & 0.048    &  3.000 & 5.525 & 0.505 & 0.206		&	2.233	&3.112&	0.171\\

       \cmidrule(){2-15}

    &  MegVii \cite{zhu2019class}+AB3DMOT \cite{Weng2020_AB3DMOT} (IROS2020)    & 0.328 & 0.585 & \underline{61} & 398 & 2 & 0.109 &  2.331 & 4.224  & 0.428  & 0.338		&	1.926	&2.891&	0.123\\
    
     &  CenterPoint \cite{yin2021center} (CVPR2021)                              & 0.445 & \underline{0.466} & {102} & \underline{278} & {1} &  \underline{0.156}  & \underline{2.026}  & \underline{4.081}  & \underline{0.383} & 0.373	&		1.601&	2.632	&0.134\\
     
     &  VoxelNext \cite{chen2023voxelnext} (CVPR2023)                            & \underline{0.480} & 0.484 & 90 & {266} & {1} &  0.106 &  2.196 & 4.562  & 0.512 &\underline{0.478}&			\underline{1.539}&	\underline{2.465}	&\underline{0.113}\\

     \cmidrule(){2-15}
     & GT position and identity        & 0.980 & 0.000 & 14 & 0 & 0 & 0.354   & 1.859  & 4.042 & 0.382 & 0.783		&	1.051	&1.976&	0.097\\
     
     &  GT position + Tracking model \cite{yin2021center}      & 0.949 & 0.000 & 14 & 0 & 21 & 0.294 &  1.939 & 4.086  &  0.400 &0.751	&		1.351	&2.401&	0.116\\

     \midrule
     \parbox[t]{3mm}{\multirow{10}{*}{\rotatebox[origin=c]{90}{Truck}}} &   MUTR3D R50 \cite{zhang2022mutr3d} (CVPRW2022)        & -0.129 & 0.886 & 334 & 1235 & 2 & 0.001 &  5.532 & 9.730  & 0.563 & 0.027		&	2.639	&4.067	&0.221\\

     &  MUTR3D R101 \cite{zhang2022mutr3d} (CVPRW2022)                                                                          & -0.083 & 0.807 & 261 & 1244 & 2 & 0.002  & 5.036  &  8.633 & 0.577 &0.035		&	2.436	&3.811&	0.212\\
     
     &  ViP3D Det\&Track \cite{gu2023vip3d} (CVPR2023)                                                                           & -0.103 & 0.945 & 293 & 1241 & \underline{0} & 0.008  & 2.657  & 4.590  & \underline{0.361} & 0.017		&	2.599	&3.989	&0.225\\
     
     &  UniAD Det\&Track \cite{uniad} (CVPR2023)                                                                                 & \underline{0.048}  & 0.723 & 119 & \underline{1205} & \underline{0} & 0.018  & 2.607  &  4.693 & 0.404 & 0.054	&		2.590	&3.978	&0.222 \\

       \cmidrule(){2-15}

    &  MegVii \cite{zhu2019class}+AB3DMOT \cite{Weng2020_AB3DMOT} (IROS2020)    & -0.146 & 0.541 & 357 & {1233} & 4 & 0.013 & 3.017 & 5.278  &  0.482  & 0.060		&	2.787	&4.536	&0.239\\
    
     &  CenterPoint \cite{yin2021center} (CVPR2021)                              & {0.004} & {0.358} & \underline{143} & 1242 & \underline{0}& 0.016& \underline{2.110}  & \underline{4.505}  & 0.455 & 0.076	&		1.841&	3.136	&\underline{0.192}\\
     
     &  VoxelNext \cite{chen2023voxelnext} (CVPR2023)                            & -0.031 & \underline{0.285} & 182 & 1252 & \underline{0} & \underline{0.023}  &  2.287 &  4.657 & 0.442 & \underline{0.085}	&		\underline{1.815}&	\underline{3.131}	&0.213\\

     \cmidrule(){2-15}
     & GT position and identity         & 0.973 & 0.000 & 38 & 0 & 0 &  0.300  & 1.966  & 4.211   & 0.408  & 0.733		&	1.309	&2.554&	0.127\\
     
     &  GT position + Tracking model \cite{yin2021center}       & 0.948 & 0.000 & 31 & 0 & 41 & 0.290  & 2.047  &  4.288 &  0.417 & 0.702		&	1.528	&2.863	&0.146 \\

     \midrule
     \parbox[t]{3mm}{\multirow{10}{*}{\rotatebox[origin=c]{90}{All}}} &   MUTR3D R50 \cite{zhang2022mutr3d} (CVPRW2022)        &0.170 & 0.607 & 1828 & 6696 & 27 & 0.042  &  3.993 & 7.151  & 0.463 & 0.152		&	2.237	&3.554	&0.178 \\

     &  MUTR3D R101 \cite{zhang2022mutr3d} (CVPRW2022)                                                                          & 0.213 & 0.550 & 1373 & 6727 & 11 &0.055 & 3.480  & 6.286  &  0.449 & 0.198		&	1.892	&3.043&	\underline{0.150}\\
     
     &  ViP3D Det\&Track \cite{gu2023vip3d} (CVPR2023)                                                                           & 0.145 & 0.636 & 1855 & 6947 & 3 & 0.056  &  2.416 &  4.404 & \underline{0.353} &0.142	&	2.044	&3.173	&0.155 \\
     
     &  UniAD Det\&Track \cite{uniad} (CVPR2023)                                                                                 & 0.195 & 0.471 & \underline{1199} & 7076 & 20 & 0.069  & 2.530  & 4.613  & 0.384 &0.180		&	2.142	&3.424	&0.169\\

       \cmidrule(){2-15}

    &  MegVii \cite{zhu2019class}+AB3DMOT \cite{Weng2020_AB3DMOT} (IROS2020)    & 0.226 & 0.320 & 1657 & 6232 & 79 & 0.089 & 2.356  & 4.412  & 0.382 & 0.227		&	2.143	&3.561	&0.168\\
    
     &  CenterPoint \cite{yin2021center} (CVPR2021)                              & \underline{0.348} & \underline{0.244} & 1622 & \underline{5090} & {5} &  \underline{0.112} & \underline{2.102}   &  \underline{4.354}&  0.413& 0.285		&	\underline{1.596}&	\underline{2.815}&	0.151\\
     
     &  VoxelNext \cite{chen2023voxelnext} (CVPR2023)                            & 0.328 & 0.263& 1639 & 5283 & \underline{2} & 0.096   & 2.134  & 4.409  &  0.426 & \underline{0.317}	&		1.669	&2.914	&0.166\\

     \cmidrule(){2-15}
     & GT position and identity        & 0.985 & 0.000 & 155 & 0 & 0 &  0.343  & 1.885  & 3.979  & 0.359 & 0.757		&	1.213&	2.316	&0.115\\
     
     & GT position + Tracking model \cite{yin2021center}      & 0.967 & 0.001 & 180 & 0 & 165 & 0.317  &  1.934 & 4.020  &  0.363 & 0.730			&1.353	&2.513	&0.125\\

    \bottomrule
    \end{tabular}
    }
  \label{tab:real_world_results_per_class}
\end{table*}

\section{More Experiments with Maps}

\begin{table*}[h]
\centering
    \caption{\yihongh{Drop of performance when removing classes of map elements from the GT map.}}
    
    \resizebox{0.9\linewidth}{!}{
    \begin{tabular}{l l c c c c}
    \toprule
     & & mAP${_f}$  $\uparrow$ & minADE $\downarrow$  & minFDE $\downarrow$  & MR $\downarrow$ \\

     \midrule  
     \parbox[t]{3mm}{\multirow{4}{*}{\rotatebox[origin=c]{90}{AgentF.}}} & with GT \eloih{rasterized} HD map                                              &0.388	&1.851	&3.875	&0.315  \\  
       & \hspace{0.5cm} without road polygons                                      &\textbf{-0.092}	&\textbf{+0.171}	&\textbf{+0.453}	&\textbf{+0.072}\\ 
       & \hspace{0.5cm} without road divider                                        &-0.001&	+0.007	&+0.018	&+0.002 \\  
       & \hspace{0.5cm} without lane divider                                      &-0.001	&+0.009	&+0.034	&+0.007 \\  
     \midrule  
     \parbox[t]{3mm}{\multirow{3}{*}{\rotatebox[origin=c]{90}{LaPred}}} & with GT \eloih{vectorized} HD map                                              & {0.760}	&{1.237}	&{2.344}	&{0.118} \\  
     & \hspace{0.5cm} without lane                                      &\textbf{-0.149}	&\textbf{+0.272}	&\textbf{+0.664}	&\textbf{+0.093}\\ 
     & \hspace{0.5cm} without lane connector                                      &-0.092	&+0.162	&+0.390	&+0.044\\ 
    \bottomrule
    \end{tabular}
    }
  \label{tab:semantic_map_imperfections}
  \vspace{+5mm}
\end{table*}

\subsection{Which map annotations are important?}
\label{subsec:mapsemantic}
In AgentFormer, maps are represented as RGB images where five semantic classes are rasterized. The first channel combines information from `lane', `road segment', and `drivable area' (i.e., road polygons) providing a broad overview of the road.
The second and third channels encode `road divider' and `lane divider' respectively, capturing finer-grained details %
of the HD maps. \yihongh{In LaPred, 'lane' and their connectors are used with a vectorized representation.}
To further study which types of annotations are important for forecasting, we remove, for each class, all of its elements from the curated maps and report in \autoref{tab:semantic_map_imperfections} the performance drop due to their absence. For rasterized representation, we identify that road polygons are especially important, while other map elements do not seem impactful. \eloih{Similarly in the vectorized representation, 'lane' that describes the high-level drivable area shows bigger importance to the forecasting performance of LaPred.} \yihongh{And we also observe that map details such as lane dividers, road dividers, and connectors are still not fully explored in both methods.}

\subsection{Online mapping method perception performance}
\label{subsec:onlinemapperf}
For the online-mapping experiments, instead of relying on ground-truth HD maps, we generate them from raw inputs.
Following the studied forecasting models \cite{uniad,yuan2021agentformer}, we represent HD maps using rasterized representation with a $100 \times 100$m receptive field around the ego car with a pixel-to-meter ratio of 0.5. Unlike HD map used in AgentFormer, we lack context on elements far away from the ego vehicle. So, to enrich the map context, we collect and combine the estimated BEV maps obtained throughout the ego car's trajectory in the same scene.
We study an explicit model (LaRa \cite{bartoccioni2022lara}) and an implicit model (SimpleBeV \cite{harley2022simple}) to estimate HD maps. SimpleBeV leads to better results but takes longer time to train due to a lower batch size and a higher memory consumption. 
Results are obtained with an image resolution of $224 \times 448$ pixels which leads to less accurate results than high definition images but with a higher FPS rate which could be a constraint for autonomous driving models. 
The calculated intersection-over-union (IoU) is the ratio of the intersection area between the predicted binarized segmentation map and the ground-truth to their union area. Results are provided in \autoref{tab:real_world_map_pred}.

Furthermore for LaPred, we leverage a state-of-the-art online \textit{vectorized} mapping method, MapTR \cite{MapTR} for predicting map elements around the ego car's field of view (60 x 30 meters). Similarly, we accumulate all the predicted map elements around the ego car in the same scene. The evaluation is based on the mAP compared to ground-truth HD map elements within the field of view, similar to the object detection task. The results are provided in \autoref{tab:real_world_map_pred_vector}.
\begin{table*}[ht]
\centering

\tabcolsep=0.11cm
    \caption{Online mapping evaluated on nuScenes validation set. BEV segmentation (IoU).}
    \resizebox{0.9\linewidth}{!}{
    \begin{tabular}{c l c c c c c c c c  c}
    \toprule
     & Method & Lane & Road segm. & Driv. area & Road div. & Lane div. & Stop line & Ped. cross. & Walkway & Mean \\ [0.5ex]

     \midrule  &   
    SimpleBeV \cite{harley2022simple} & 0.546 & 0.690 & 0.672 & 0.324 & 0.430 & 0.281 & 0.325 & 0.401 & 0.458 \\
     &  LaRa \cite{bartoccioni2022lara} & 0.465 & 0.610 & 0.599 & 0.230 & 0.317 & 0.159 & 0.200 & 0.310 & 0.361 \\
    \bottomrule
    \end{tabular}
    }
  \label{tab:real_world_map_pred}
\end{table*}

\begin{table*}[ht]
\centering

\tabcolsep=0.11cm
    \caption{Performance of vectorized online mapping MapTR (LiDAR + Camera) \cite{MapTR} on nuScenes.}
    \resizebox{0.7\linewidth}{!}{
    \begin{tabular}{c l c c c }
    \toprule
    Dataset & AP\_ped & AP\_divider & AP\_boundary & mAP \\ [0.5ex]

    \midrule  
    nuScenes Train & 92.0 & 97.4 & 94.7 & 94.7 \\
     \midrule  
    nuScenes Validation &  56.5 & 61.8 & 70.1 & 62.8\\
    \bottomrule
    \end{tabular}
    }
  \label{tab:real_world_map_pred_vector}
\end{table*}

\subsection{Imperfections from agent or neighbors}
\yihongh{Motion forecasting methods model both the agent of interest's past trajectory and its neighbor's trajectories. We study here the impact of imperfections in both information. Concretely, we inject localization errors (+/- 2 meters) into the the past trajectories and evaluate the drop of performance compared to curated inputs. From \autoref{tab:agent_nei_noise}, we observe the localization errors from the agent of interest itself shows bigger impact on the forecasting performance.}

\subsection{Training with synthetic data augmentation}
\label{subsec:dataaugumentation}
\begin{table}[h]
\centering
    \caption{\yihongh{Finetuning LaPred with data augmentation. The data augumentation is a mixture (Mix) of FP, FN, IDS and Localization error  (Loc. Error) of three different probabilities: 10\%, 30\% and 50\%. The fine-tuning is conducted on the tracking results on the trainset and test on the validation of nuScenes Prediction.}}
    
    \resizebox{\linewidth}{!}{
    \begin{tabular}{l c c c c c}
    \toprule
    Training input & Testing input & mAP${_f}$  $\uparrow$ & minADE $\downarrow$  & minFDE $\downarrow$  & MR $\downarrow$ \\

     \midrule  
     \multirow{16}{*}{Ground truth} & GT  & 0.760 & 1.237 & 2.344 & 0.118 \\  
       &  VoxelNext                                     &  0.317 & 1.669 & 2.914 & 0.166\\ 
       &  UniAD                                        &0.180 &2.142 &3.424 & 0.169 \\  
       & MUTR3D R101                                      &0.198 & 1.892 & 3.043 & 0.150\\ 
       & {10\% FN} & & & & \\
       & {30\% FN} & & & & \\
       & {50\% FN} & & & & \\
       
       & {10\% FP} & & & & \\
       & {30\% FP} & & & & \\
       & {50\% FP} & & & & \\
       
       & {10\% IDS} & & & & \\
       & {30\% IDS} & & & & \\
       & {50\% IDS} & & & & \\
       
       & {10\% Loc. Error} & & & & \\
       & {30\% Loc. Error} & & & & \\
       & {50\% Loc. Error} & & & & \\
     \midrule   

       \multirow{3}{*}{10\% Mix} &  VoxelNext                                     & -0.007	&+0.147	&+0.053&	-0.002\\ 
       &  UniAD                                        &+0.013	&-0.041	&-0.158	&-0.015 \\  
       & MUTR3D R101                                     &+0.015	&-0.016&	-0.154	&-0.006\\ 

       10\% FN & 10\% FN & & & & \\
       10\% FP & 10\% FP & & & & \\
       10\% IDS & 10\% IDS & & & & \\
       10\% Loc. Error & 10\% Loc. Error & & & & \\

    \midrule   
      
      \multirow{3}{*}{30\% Mix} &  VoxelNext                                    & -0.014	&+0.293	&+0.207	&+0.014\\ 
       &  UniAD                                        &+0.005	&-0.117	&-0.234&	-0.006\\  
       & MUTR3D R101                                      &+0.007	&+0.067	&-0.002	&+0.014\\
       30\% FN & 30\% FN & & & & \\
       30\% FP & 30\% FP & & & & \\
       30\% IDS & 30\% IDS & & & & \\
       30\% Loc. Error & 30\% Loc. Error & & & & \\

    \midrule   
       \multirow{3}{*}{50\% Mix} &  VoxelNext            &-0.019	&+0.462	&+0.368	&+0.023\\ 
       &  UniAD                                        &-0.007&	+0.093	&+0.030	&+0.019 \\  
       & MUTR3D R101                                    & -0.013&	+0.236	&+0.221	&+0.036\\
       50\% FN & 50\% FN & & & & \\
       50\% FP & 50\% FP & & & & \\
       50\% IDS & 50\% IDS & & & & \\
       50\% Loc. Error & 50\% Loc. Error & & & & \\

     \midrule   
     \xyhh{100\% Loc. Errors} & \xyhh{100\% Loc. Errors} & 0.619	&2.005	&3.201	&0.189\\
    \bottomrule
    \end{tabular}
    }
  \label{tab:train_da}
\end{table}

\yihongh{We train with a mixture of different data augmentation (FP, FN, and IDS) to the past trajectories with different probabilities, showing that simple data augmentations cannot improve the forecasting performance with real-world imperfections.}

\yihongh{As for implementation details for training with imperfections. For synthetic data augmentation, we randomly add FP, FN and IDS to the past trajectories. We show that simple synthetic data augmentation is not helper neither. The above observations indicate that directly finetuning with real-world inputs cannot close the performance gap compared to curated inputs.}
\yihongh{It is more complicated with real-world inputs since we need to match real-world past trajectories with ground-truth future trajectories. We finetune the model with a mixture of ground-truth past trajectories (when real-world inputs are unavailable) and real-world inputs. More precisely, for each ground-truth agent, we match at t=0 with the closest real-world input if it is less than 2m away (the threshold used in the metrics) based on their Euclidean distance. Once they are matched, we extract the past of this real-world input as the past trajectory for the agent and learn to predict the matched ground-truth future trajectory. Knowing that since the real-world inputs are sometimes missing for certain agents (FN@t=0), we complete them with ground-truth trajectories. We also note that the training is with nuScenes training set and evaluate on the validation set because over-fitting to the validation set is meaningless. In practice, the environment where the autonomous driving car is exposed is ever-changing.}

\begin{table}[t]
\centering

    \caption{Performance of LaPred \cite{yuan2021agentformer} given perturbations in agent-of-interest's or neighbors' trajectories.}
    \resizebox{\linewidth}{!}{
    \begin{tabular}{@{}l c c c c@{}}
    \toprule
    Setting & mAP${_f}$  $\uparrow$ & minADE $\downarrow$  & minFDE $\downarrow$  & MR $\downarrow$ \\

     \midrule  
      Ground truth                             &0.760	& 1.237	& 2.344	& 0.118   \\  
      Agent Loc.Error                           &0.176	& 4.991	& 6.450	& 0.520 \\
      Neighbor Loc.Error                       &0.744	     & 1.291	& 2.474	& 0.125 \\ 
    \bottomrule
    \end{tabular}
    }
  \label{tab:agent_nei_noise}
\end{table}

\section{Dataset and Metric Details}
\subsection{Dataset}
We evaluate our models on the nuScenes dataset \cite{nuscenes}, which comprises a thousand 20-second urban scenes recorded in Boston and Singapore. Each scene provides data from multiple cameras, LiDAR, and radars, along with high-definition maps and 3D annotations at a frequency of 2 Hz. To assess the tracking and forecasting performances, we employ the official train - validation - test splits from the nuScenes prediction challenge with a past context defined as a 2-second history and a future horizon of up to 6 seconds into the future. According to the challenge, we remove the `emergency police' and `construction vehicle' since it only concerns a couple of examples and it does not overly impact the metrics. 

\subsection{Forecasting metrics}
The abbreviations of the metrics used for the forecasts are described in more detail below.

\begin{itemize}[leftmargin=.5cm,itemsep=0cm]
    \item $\text{minADE}_k$: best among $k$ forecasted trajectories in terms of the Average euclidean Distance Error (ADE) with the ground truth. Unless otherwise specified, $k=5$ modes for AgentFormer and $k=10$ for LaPred.
    \item $\text{minFDE}_k$: best among $k$ forecasted trajectories in terms of the Final euclidean Distance Error (FDE) with the ground truth. Unless otherwise specified, $k=5$ modes for AgentFormer and $k=10$ for LaPred.
    \item $\text{MR}_{k@x}$: stands for Miss Rate. It is the proportion of matched samples where none of the $k$ forecasted trajectories are within $x$ meters of the ground truth. Unless otherwise specified, $k=5$ modes for AgentFormer, $k=10$ for LaPred, and $x=4$m by default.
\end{itemize}

\subsection{Tracking metrics}
\label{subsec:metrics}
We detail here the two tracking metrics 
Multiple Object Tracking Accuracy (MOTA) \cite{bernardin2008evaluating} and Multiple Object Tracking Precision (MOTP).

\begin{itemize}
    \item Multiple Object Tracking Accuracy (MOTA) combines FP, FN and IDS  as follows $\text{{MOTA}} = 1 - \frac{{\text{{FP}} + \text{{FN}} + \text{{IDS}}}}{{\text{{GT}}}}$ where GT is the number of GT objects.
    \item Multiple Object Tracking Precision (MOTP) quantifies the average positional precision over matched objects by calculating the average distance between the predicted boxes and their corresponding ground-truth positions: $\text{{MOTP}} = \frac{{\sum_{{i=1}}^{{N}} \sum_{{j=1}}^{{M_i}} d_{{ij}}}}{{\sum_{{i=1}}^{{N}} M_i}}$ where $N$ is the number of frames, $M_i$ is the number of associations in frame $i$, and $d_{ij}$ is the Euclidean distance between the centers of the predicted and ground-truth bounding boxes. %
\end{itemize}
\begin{table*}
\centering
\tabcolsep=0.11cm
    \caption{Summary of considered tracking methods.}
    \resizebox{0.9\linewidth}{!}{
    \begin{tabular}{l l c c l}
    \toprule
     \multicolumn{1}{l}{\textbf{Method}} & Conference & Camera-based & Lidar-based & Type of tracking \\ 
    \midrule
     GT position and identity & --- & --- & --- & Ground-truth tracking \\ 
     GT position + Tracking model \cite{yin2021center} &  --- & --- & --- & Simple tracking \\
     MUTR3D R50 \cite{zhang2022mutr3d} & CVPRW 2022 & \cmark & \xmark & Joint detection and tracking \\ 
     MUTR3D R101 \cite{zhang2022mutr3d} & CVPRW 2022 & \cmark & \xmark & Joint detection and tracking \\ 
     ViP3D Det\&Track \cite{gu2023vip3d} & CVPR 2023 & \cmark & \xmark & Forecasting-aware tracking \\ 
     UniAD Det\&Track \cite{uniad} & CVPR 2023 & \cmark & \xmark & Planning-aware tracking \\
     MegVii \cite{zhu2019class} + AB3DMOT \cite{Weng2020_AB3DMOT} & IROS 2020 & \xmark & \cmark & Separate Detection and Tracking \\
     CenterPoint \cite{yin2021center} & CVPR 2021 & \xmark & \cmark & Joint detection and tracking \\ 
     VoxelNext \cite{chen2023voxelnext} & CVPR 2023 & \xmark & \cmark & Joint detection and tracking \\
    \bottomrule
    \end{tabular}
    }
  \label{tab:tracking_methods}
\end{table*}

\section{Overview of the Models}
Our study involves the use of several state-of-the-art detection, tracking, and forecasting models. Here is a more detailed description of the used models. \autoref{tab:tracking_methods} summarizes the detection and tracking models.

\subsection{Perception LiDAR-based models}
\begin{itemize}[leftmargin=0.5cm]
    \item MegVii \cite{zhu2019class} performs 3D detection in point clouds with sparse 3D convolutions. We then feed these detections to AB3DMOT \cite{Weng2020_AB3DMOT} that is a simple real-time 3D tracking method based on combining Kalman filtering and Hungarian matching. 
    \item CenterPoint \cite{yin2021center} first detects centers of objects and then regresses other attributes (size, orientation, etc.). The identity matching is conducted at the center level with greedy closest-point matching. 
    \item VoxelNext \cite{chen2023voxelnext} divides a point cloud into a 3D voxel partition and transforms a group of points within each voxel into a unified representation that is finally processed by a region proposal network.
\end{itemize}

\subsection{Perception vision-based models}
\begin{itemize}[leftmargin=0.5cm]
    \item ViP3D Det\&Track \cite{gu2023vip3d} and UniAD Det\&Track \cite{uniad} both use query-based transformer architectures to output 3D bounding boxes and tracking ids by inputting 2D images from 6 cameras surrounding the ego vehicle.
    \item MUTR3D \cite{zhang2022mutr3d} is a multi-camera based 3D object tracking method. It leverages 3D track queries and 3D-to-2D transformations to link 3D objects with their corresponding 2D objects in images. It also uses a set prediction loss to discard the non-maximum suppression as post processing.
\end{itemize}

\subsection{Motion forecasting models}
\label{subsec:forecastingmodels}
\begin{itemize}[leftmargin=0.5cm]
\item  AgentFormer \cite{yuan2021agentformer} formulates the forecasting problem as the modeling of all surrounding agents conditioned on their past trajectories and contextual road elements. It is based on a Conditional Variational AutoEncoder \cite{cvae} framework, and takes the contextual road inputs in the form of a \textit{rasterized} semantic map (lanes, dividers).
\item \yihongh{LaPred \cite{kim2021lapred} predicts per-agent future trajectories leveraging the closest \textit{vectorized} lane information and past trajectories of neighboring agents. The past trajectory of the agent of interest, the nearby lane information, and the past trajectories of neighbors are encoded with a 1D convolution and LSTM module and then combined together. This combined feature enforces the use of \textit{vectorized} map information as well as the behavior of neighbor agents, building a strong baseline even with a simple yet efficient MLP-based trajectory decoder.}
\item ViP3D \cite{gu2023vip3d} leverages tracking and detection queries (hidden embeddings) to perform new-object discovery and encode object past history, respectively. The remained tracking queries at $t=0$, which encode the past information and interactions between agents, are used to decode the future trajectories with fully-connected layers using classic regression-based losses. The vectorized map information \cite{vectornet} from HD maps is used.
\item UniAD \cite{uniad} proposes an end-to-end detection, tracking, online-mapping, forecasting, and planning model interacting with a bird's-eye-view (BEV) embedding \cite{li2022bevformer}. The forecasting module of UniAD has an attention-based structure taking the perception (detection and tracking) queries as inputs. The future trajectories are further refined by a goal-point prediction attention module and a non-linear kinematic model \cite{nuplan} that respects physics.
\end{itemize}

\begin{figure*}[h]
\centering
\begin{subfigure}{0.24\linewidth}
\includegraphics[trim={0cm 1.8cm 0 2.0cm},clip, width=\linewidth]{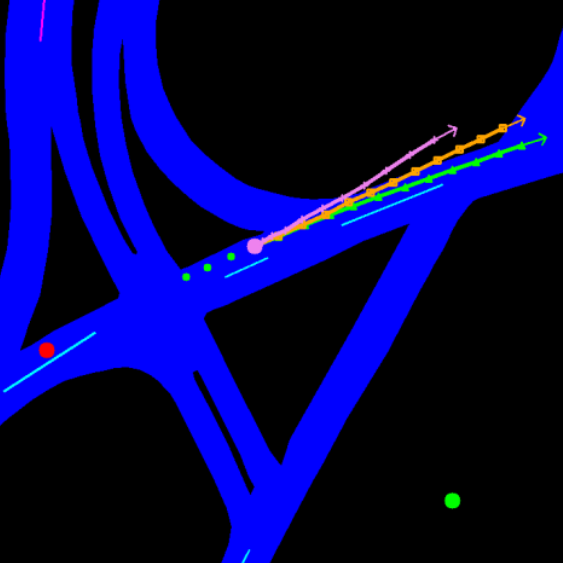} 
    \vspace{-0.6cm} 
  \caption{FN\vspace{-0.2cm}}
\end{subfigure}
\centering
\begin{subfigure}{0.24\linewidth} 
\includegraphics[trim={0cm 1.8cm 0 2.0cm},clip, width=\linewidth]{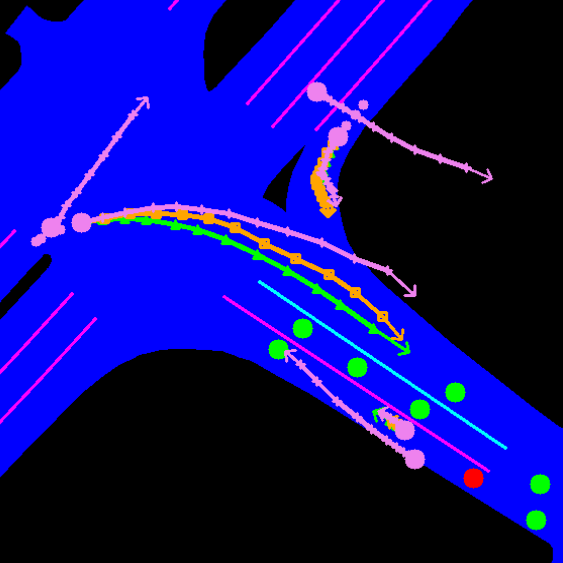}
    \vspace{-0.6cm} 
  \caption{FP\vspace{-0.2cm}}
\end{subfigure}
\centering
\begin{subfigure}{0.24\linewidth}
\includegraphics[trim={0cm 1.8cm 0 2.0cm},clip, width=\linewidth]{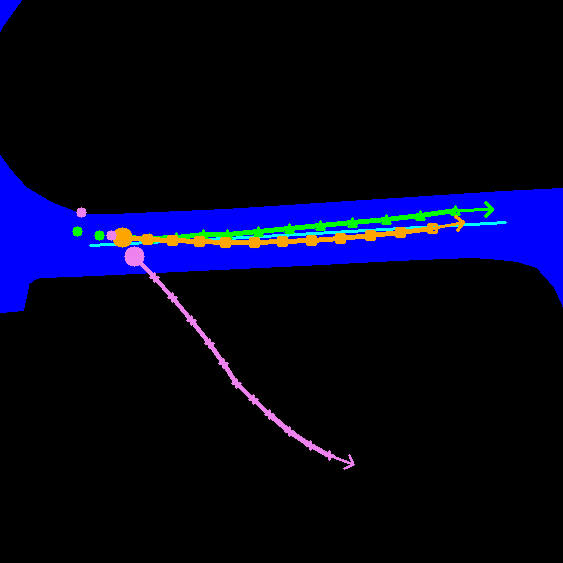}
    \vspace{-0.6cm} 
  \caption{Localization error\vspace{-0.2cm}}
\end{subfigure}
\centering
\begin{subfigure}{0.24\linewidth}
\includegraphics[trim={0cm 1.8cm 0 2.0cm},clip, width=\linewidth]{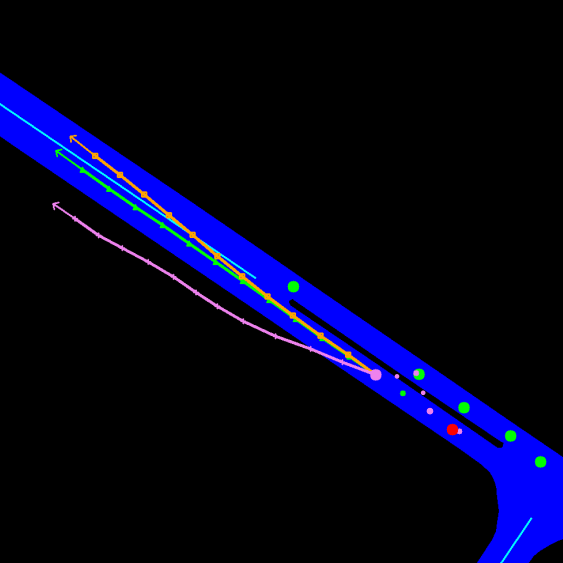}
    \vspace{-0.6cm} 
  \caption{IDS\vspace{-0.2cm}}
\end{subfigure}
\caption{(a) Lost past trajectory causes imprecise forecasting. (b) False positives affect the predicted trajectory. (c) Imprecise past trajectory causes impactful forecasting errors. (d) Identity switching modifies the past trajectory thus creating a different forecasting outcome. (pink) Past trajectory and future forecasts \cite{yuan2021agentformer} with perception inputs \cite{Weng2020_AB3DMOT, zhu2019class}; (orange) future forecasts with curated past inputs; (red) ego car; (green) curated agents and trajectories; (blue) drivable area; (cyan) road lines; (magenta) lane boundaries.}
\label{fig:visu}
\vspace{-6mm}
\end{figure*}

\section{Qualitative Visualizations}
\xyhh{In \autoref{fig:visu}, we visualize imperfections from the perception upstream tasks \cite{Weng2020_AB3DMOT, zhu2019class} and show how they are able to modify the prediction of motion forecasting \cite{yuan2021agentformer} (pink v.s.~orange).}
